# Supplementary material for: M2C: Towards Automatic Multimodal Manga Complement
Source: arXiv:2310.17130 source file (2023-10-26)
Supplement: Supplementary file 1 [file appendix.tex]

\section{Appendix}

\begin{figure}[!htp]
\begin{center}
\includegraphics[width=1\linewidth]{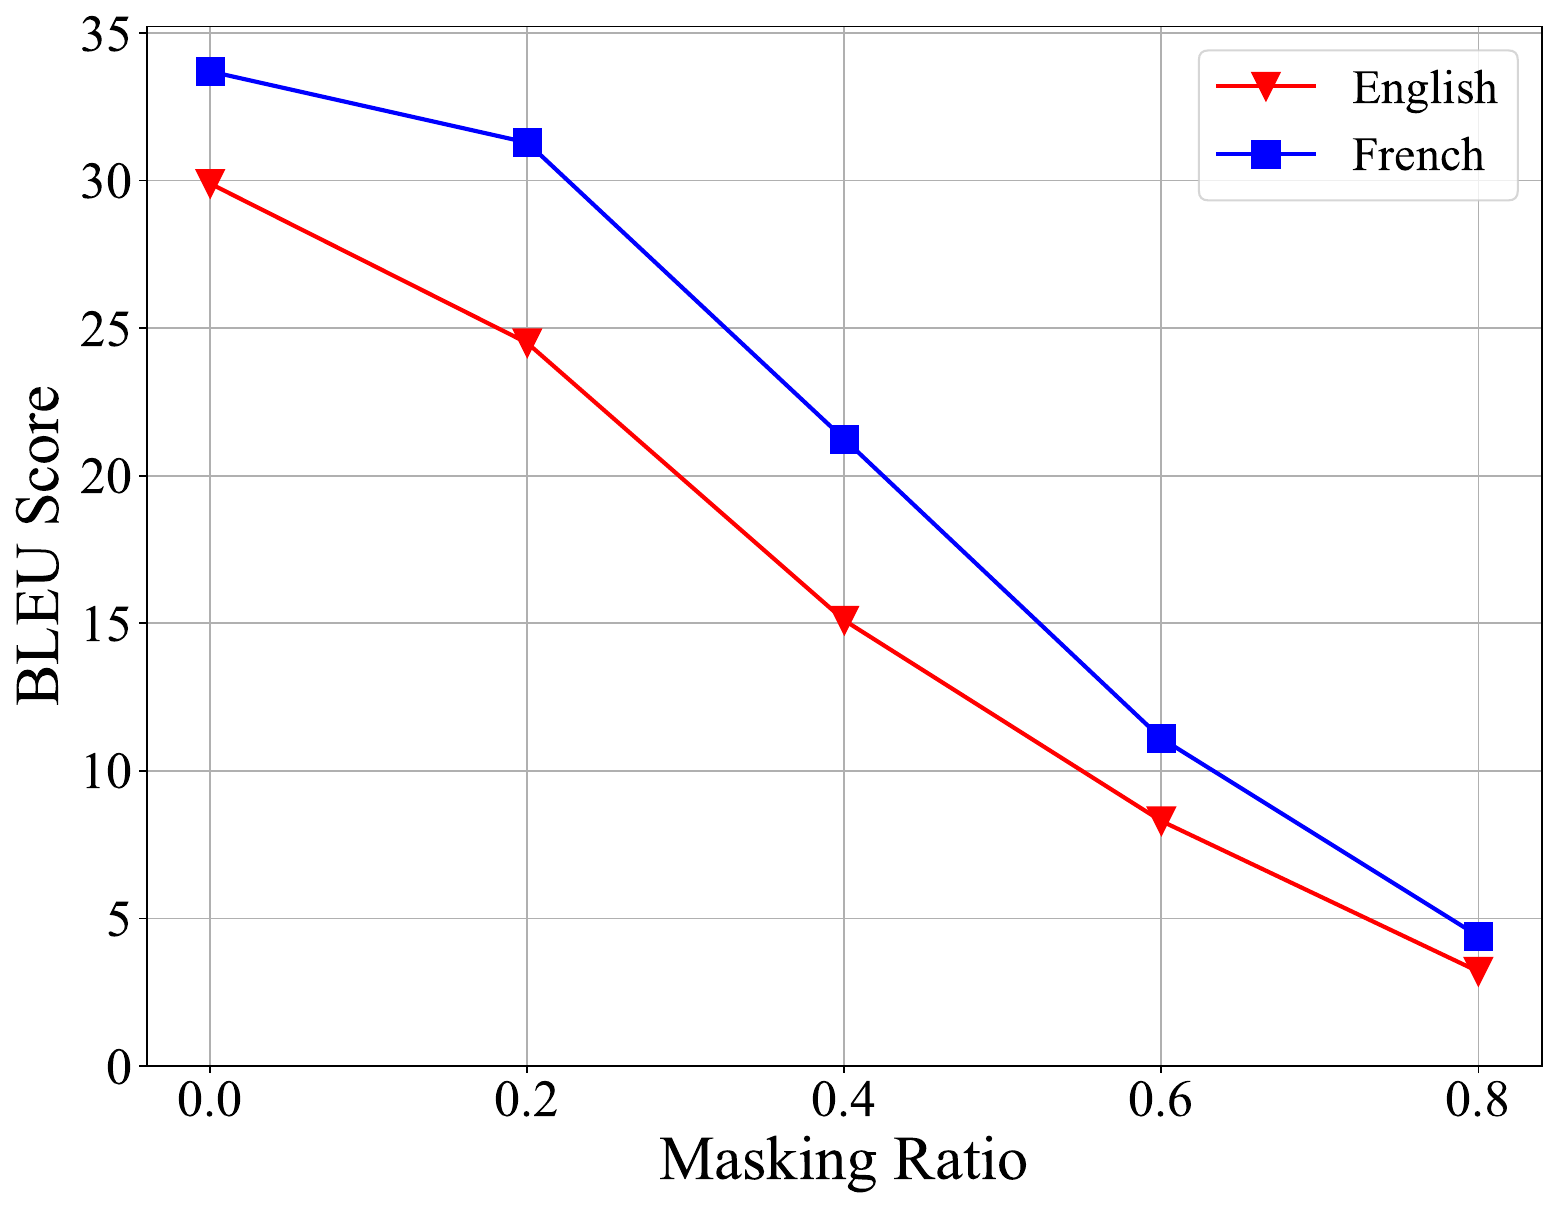}
% \vspace{-3mm}
\caption{BLEU results of \ourmethod{} under different masking ratios on the input data.}
% source description in English, together with its different .}
\label{fig:rate}
% \vspace{-5mm}
\end{center}
\end{figure}

\subsection{Results of Different Masking Ratios.}
As shown in Fig.~\ref{fig:rate}, we analyze the effectiveness of visual context when using different masking ratios on the source corpus. we report the results of two languages.
First, when the ratio of masking increases, BLEU scores drop. Second, the performance gap between English and French is larger
when the mask ratio is between 20\% and 40\%,
which shows that the visual information improves the robustness of the model and it has different impact on different languages.
Third, when the mask ratio is larger,
the results on all settings degrade.
When the mask ratio is set as 80\%, the results of English are close to French.
It is also reasonable,
because most tokens in each source corpus are masked and it is difficult to generate well for both languages under these extreme scenarios.
